# Supplementary material for: Deterministic transfer of optical-quality carbon nanotubes for atomically defined technology
Source: arXiv:2012.01741 ancillary file (2020-12-03)
Supplement: Supplementary file 1 [file anthracene-transfer-SI.pdf]

**Supplementary Information**

# Deterministic transfer of optical-quality carbon nanotubes for atomically defined technology

Keigo Otsuka[1], Nan Fang[1], Daiki Yamashita[2], Takashi Taniguchi[3], Kenji Watanabe[4], Yuichiro K. Kato[1,2,*]

[1]Nanoscale Quantum Photonics Laboratory, RIKEN Cluster for Pioneering Research, Saitama 351-0198, Japan
[2]Quantum Optoelectronics Research Team, RIKEN Center for Advanced Photonics, Saitama 351-0198, Japan
[3]International Center for Materials Nanoarchitectonics, National Institute for Materials Science, Ibaraki 305-0044, Japan
[4]Research Center for Functional Materials, National Institute for Materials Science, Ibaraki 305-0044, Japan

* email: yuichiro.kato@riken.jp

## S1. Photoluminescence measurements during nanotube transfer

We use a homebuilt micro-photoluminescence (PL) measurement system to characterize carbon nanotubes (CNTs). To facilitate the transfer process, reflectivity of a laser beam and a coaxial wide-field LED illumination, as well as PL from CNTs are simultaneously monitored in real time. For example, the laser reflectivity provides the precise position of the receiving substrate in three coordinates. When using a transparent stamp, the reflectivity shows an interference pattern while approaching the substrate (Figure S1a). PL is monitored to non-destructively locate CNTs, identify the chirality, and capture changes in the surrounding environment of the CNTs. Note that we use a closed-loop translation stage to move the substrate, but an open-loop stage for the stamp. The reproducibility of the open-loop stage predominantly limits the position accuracy of the transfer process.

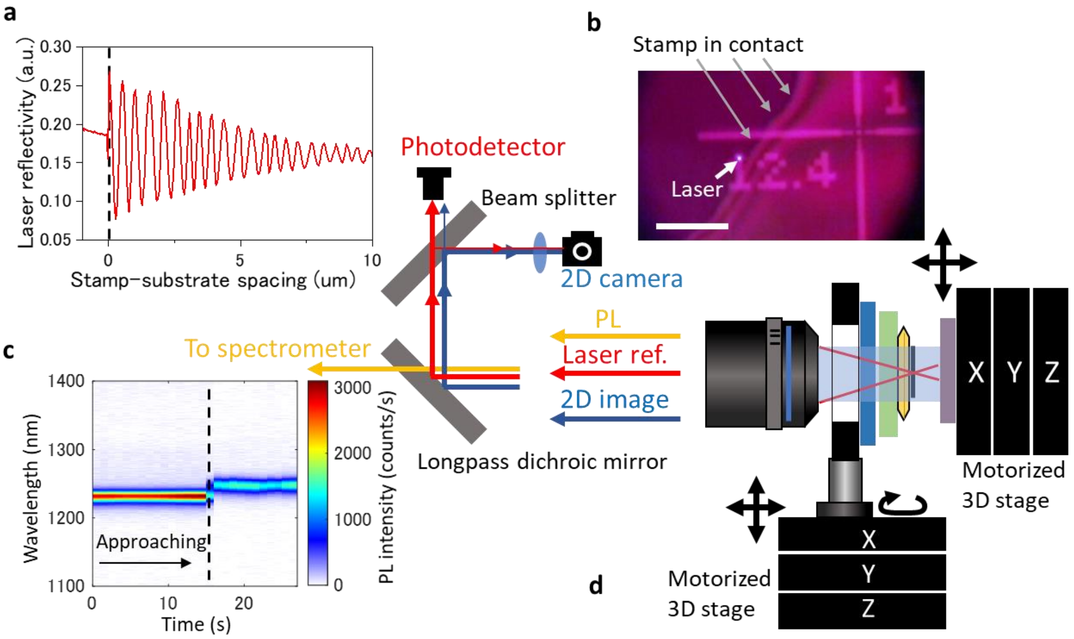


**Figure S1 | Overview of the anthracene-assisted transfer system incorporated in a micro-PL setup. a**, Reflectivity of the laser beam as a function of the spacing between a stamp and a substrate. As the stamp approaches, the amplitude of interference increases and becomes stable after the contact. **b**, Wide-field optical image of the substrate surface. The left half is in contact with the stamp. Scale bar is 20 µm. **c**, Transition of PL spectra of an air-suspended CNT while approaching an anthracene crystal to the CNT. Dashed line represents the contact of the CNT and the anthracene crystal, which induces a redshift of the emission spectra. **d**, Schematic of the transfer system in the optical setup that allows for in-situ confocal PL measurements and reflection imaging.

## S2. Crystal growth of anthracene by in-air sublimation

We employ a simple crystal growth technique, in which the temperature at a growth substate is controlled by the distance to a heated substrate with molecular powder sources [1]. The crystals are grown through sublimation in air. We find that a coating of glass slides with marker ink (blue in Figure S2a) suppresses the nucleation of anthracene crystals, which leads to the growth of large-area and thin crystals. The (001) plane of the crystals is in contact with CNTs during the transfer.

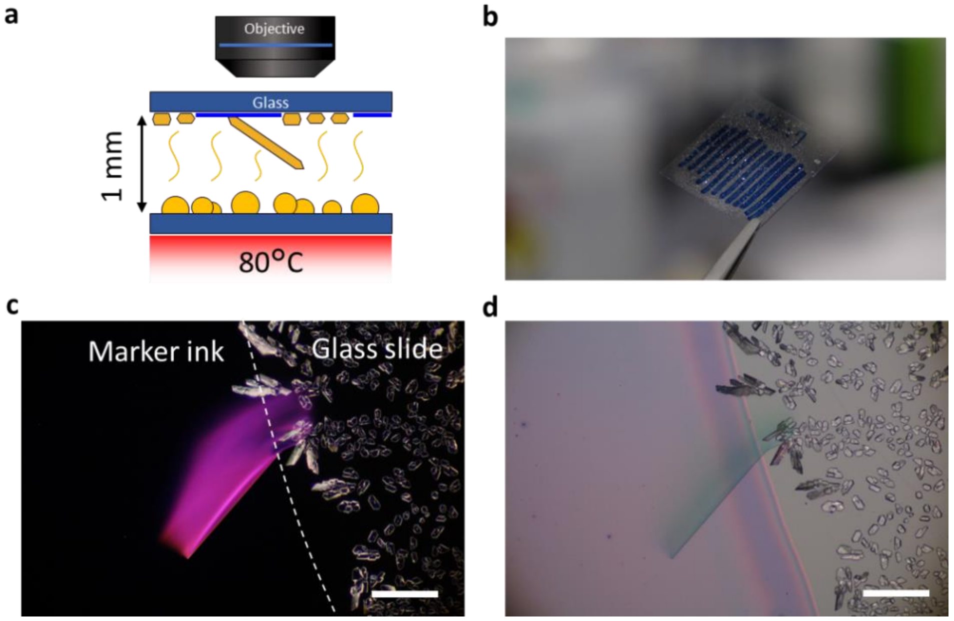


**Figure S2 | Anthracene crystal growth. a**, Schematic for crystal growth of anthracene in air. **b**, Photograph showing a glass slide after the crystal growth. Blue lines are drawn with a commercially available marker, on which the nucleation of crystals is suppressed. **c**,**d**, Optical micrographs of anthracene crystals under dark-field (**c**) and bright-field (**d**) illumination. Scale bars are 100 µm.

## S3. Diameter dependence of the transfer efficiency

Unlike the polymer-mediated transfer that involves wet etching of the growth substrates [2], the overall transfer efficiency of the dry stamping method is far less than 100%. Interestingly, chirality distribution is different for the as-grown suspended CNTs and the transferred CNTs (Figure S3a). Note that the transferred CNTs are grown on a flat $SiO_2$/Si surface from unpatterned iron catalyst. By comparing the chirality distribution between the as-grown and transferred samples (Figure S3b), we find a strong diameter dependence in the transfer efficiency (Figure S3c). As the transfer efficiency for the thinnest CNTs is obviously <100%, the efficiency for the CNTs with the diameter of ~1.2 nm or more should be <1%. Considering the crystalline nature of the anthracene stamp, there also

could be a chiral angle dependence, as well as a tube orientation dependence. The current results show a slight dependence on the chiral angle, but further study is needed.

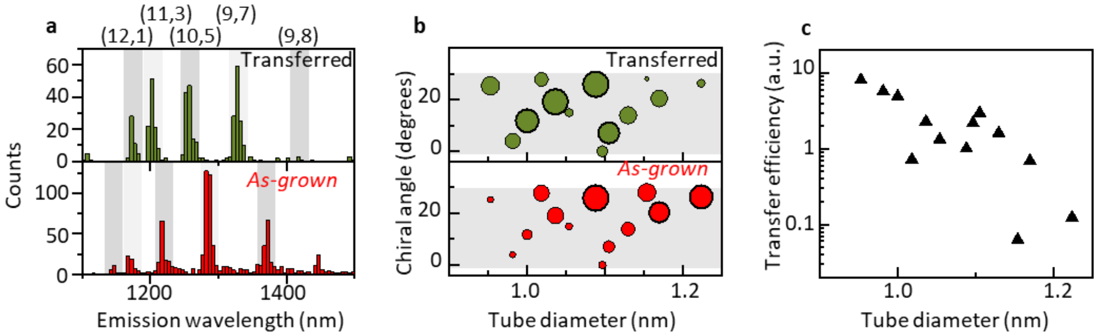


**Figure S3 | Chirality dependence of CNTs transferred via anthracene crystals. a**, Histograms of emission wavelengths for the CNTs on PMMA or suspended over trenches excited at 790 (top) and 780 nm (bottom), respectively. **b**, Chirality distribution as a function of tube diameter and chiral angle for transferred (top) and as-grown (bottom) CNTs. The area of the circles represents the population. In total, the chiral indices of 771 and 1307 tubes are assigned for the transferred and as-grown samples, respectively. **c**, Transfer efficiency *versus* tube diameter, where ratios of the abundance of transferred CNTs to as-grown CNTs in **b** are plotted.

## S4. Length of transferred CNTs on polymer

The transferred CNTs shown in Figures 3–5 and Figure S3 are grown simultaneously with the as-grown suspended ones using similar catalyst (evaporated iron). The length of those CNTs should therefore be more or less the same. In SEM and PL images in Figure S4, the typical length of the transferred CNTs is 1–5 μm and similar to those suspended over trenches. We also did not find excessive bundle formation of the transferred CNTs, indicating that the PL intensity comparison between the as-grown suspended CNTs and the transferred CNTs is not biased much by the tube length difference.

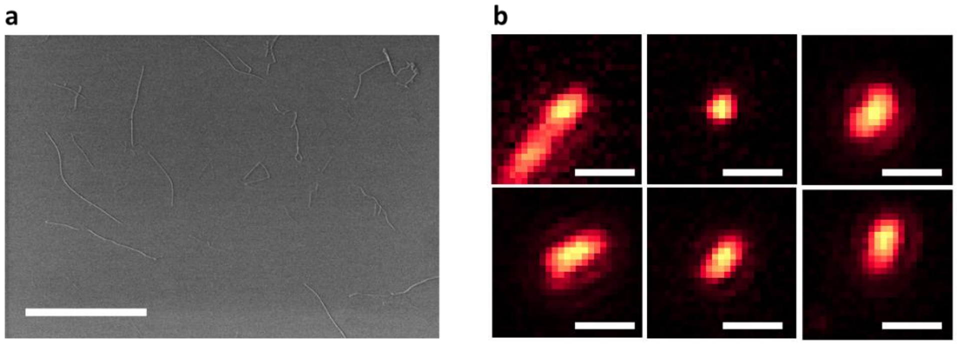


**Figure S4 | Images of transferred CNTs on polymer. a**, SEM image of transferred CNTs on PMMA. CNTs are originally grown on flat a $SiO_2$/Si substrate and randomly orientated. **b**, Typical PL images of the CNTs. Scale bars in **a** and **b** are 5 and 2 μm, respectively.

## S5. Changes to PL spectra before and after anthracene contact

We have checked that PL of CNTs is not significantly quenched by the contact with anthracene crystals. Figure S5 shows PLE maps of the same air-suspended CNT before and after the anthracene contact, which were measured through a glass/PDMS/anthracene stamp. The PL trace of this CNT during the contact formation is found in Figure S1c. The contact with anthracene induced $E_{11}$ and $E_{22}$ redshifts as well as a slight spectral broadening. The integrated PL intensity at the resonance is $2.01\times10^4$ and $1.83\times10^4$ counts/s before and after the contact, respectively. Although the collection efficiency of nanotube PL can be changed by placing materials with a high refractive index on top of the CNTs, the reduction of the PL intensity is insignificant for performing deterministic transfer of CNTs on anthracene under *in-situ* PL monitoring.

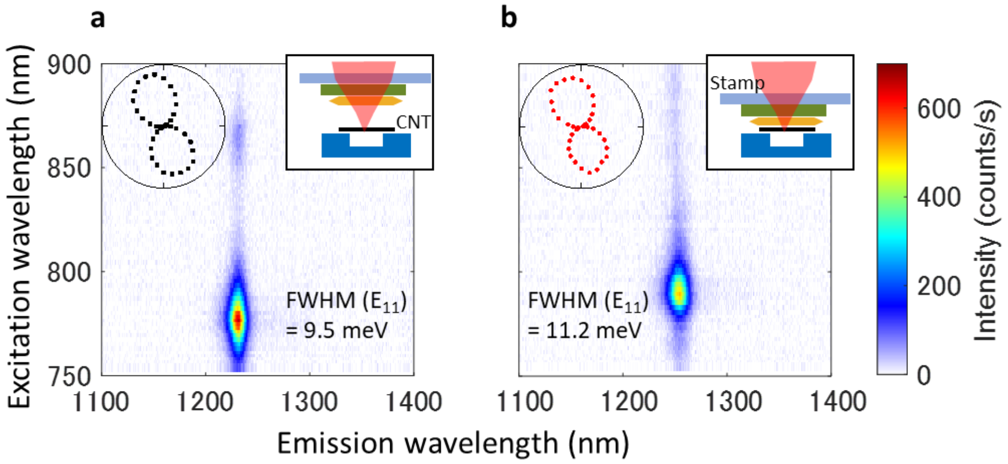


**Figure S5 | Spectral tracing of a CNT. a**,**b**, PLE maps of the same CNT before (**a**) and after (**b**) the contact with an anthracene crystal. Inset: Polarization angle-dependent PL intensity. The configuration of the sample and measurement is also shown at the top right. $P$ = 10 µW.

## S6. Statistics of PL properties for various CNT samples

In addition to Figure 3a, we have performed statistical PL measurements for two more samples: CNTs on anthracene and on $SiO_2$/Si with $P$ = 100 µW. In Figure S6a, histograms of $\log_{10}(I_{PL})$ are shown for each sample. Note that the excitation power here is much larger than that used in Figure 3a ($P$ = 5 µW), and PL enhancement factors are smaller due to efficient exciton-exciton annihilation in high PL efficiency samples. The detector noise is centered at 0 counts/s and follows a normal distribution in linear scale, but in log scale, $\log_{10}(I_{PL})$ of the noise peaks at ~3 due to uneven binning width. Similarity of the frequency corresponding to noise indicates that the density of CNTs in each sample are comparable. $I_{PL}$ of all the samples above the noise level is well fitted with a log-normal distribution (solid lines). $I_{PL}$, at which the relative frequency is $10^{-3}$ for each sample, is indicated by the vertical lines in Figure S6a. The PL intensity of the CNTs on anthracene is close to that on polystyrene, while that on $SiO_2$/Si lies between the as-grown CNTs on

quartz and the transferred CNTs on PMMA. Consistent with the previous study [3], the removal of the strong interaction with growth substrates suppresses exciton quenching, but polar substrates have stronger quenching effect than polymers.

Spectral linewidths of each sample follow a normal distribution (Figure S6b). When we fit the emission spectra of the three types of CNTs with a Voigt function, Lorentzian (related to exciton dephasing) and Gaussian components (related to inhomogeneity) can be obtained (Figure S6c,d).

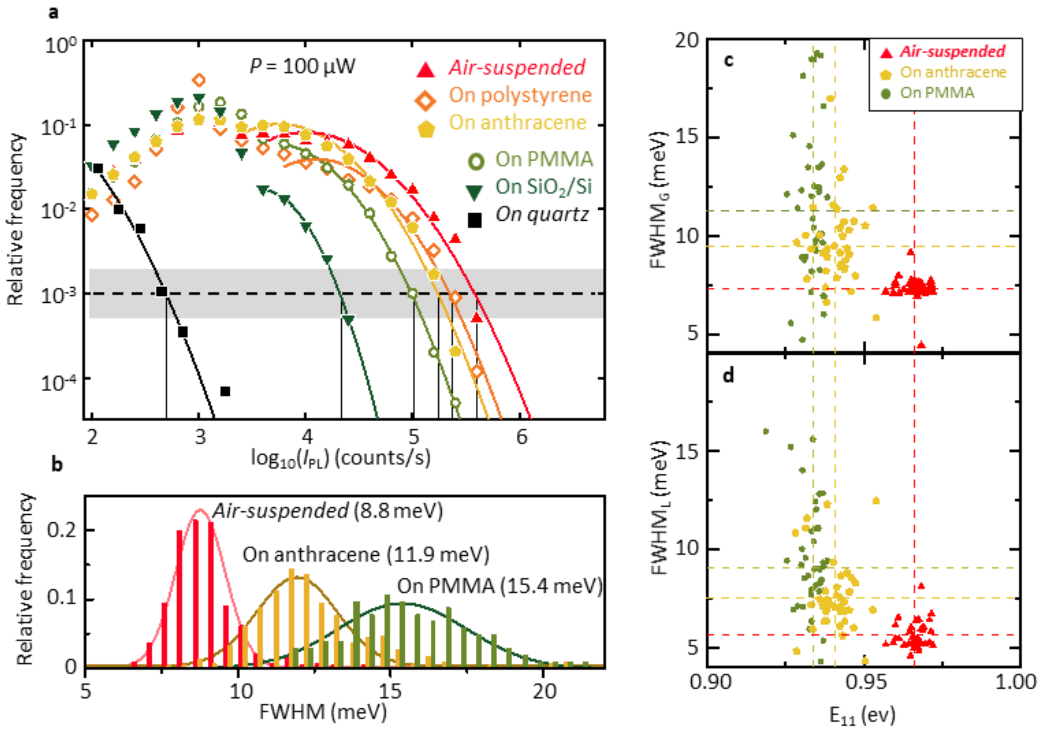


**Figure S6 | Statistical study on optical quality of various CNT samples. a**, Histograms of $\log_{10}(I_{PL})$ at $P$ = 100 µW for six types of CNTs. Peaks around $\log_{10}(I_{PL})$ = 3 originate from detector noise, and the other regions are fitted by log-normal distributions (solid lines). The frequency range $5\times10^{-2}$ to $2\times10^{-3}$ is shown in gray. **b**, Histograms of PL linewidths for three types of CNTs. Solid lines represent Gaussian fits. The sample name in Italic represent as-grown CNTs; otherwise, the CNTs are transferred *via* anthracene. **c**,**d**, Full width at half maximum (FWHM) of Gaussian components (**c**) and Lorentzian components (**d**) of the Voigt function fitting for PL spectra of three types of CNTs. Dashed lines represent the averages.

## S7. PL intensity widely ranges due to stochastic quenching sites

As shown in Figure S6, the PL intensity of individual CNT follows a log-normal distribution, and ranges over a few orders of magnitude even among as-grown suspended CNTs over the trenches with similar widths. As the chance of quenching site creation during CVD should be equal for all CNTs, the density of quenching sites in a nanotube is

expected to follow a normal distribution (or a Poisson distribution). The probability $f$ for having $\lambda$ quenching defects in a nanotube can be written as

$$f(\lambda) = \frac{1}{\sqrt{2\pi}\sigma}\exp\left(-\frac{(\lambda - N)^2}{2\sigma^2}\right), \qquad \text{(S1)}$$

with $N$ and $\sigma$ being the average number of quenching sites and its standard deviation, respectively. As shown in Figure S6, when the frequency $g$ of a CNT with $I' \equiv \ln(I_{PL})$ follows

$$g(I') = \frac{1}{\sqrt{2\pi}\alpha\sigma}\exp\left(-\frac{(I' - I'_N)^2}{2\alpha^2\sigma^2}\right) \qquad \text{(S2)}$$

with $I'_N$ being the average of $\ln(I_{PL})$, it implies that $I_{PL}$ of a CNT with $\lambda$ quenching sites is

$$I_{PL} = I_0 \exp(-\alpha\lambda), \qquad \text{(S3)}$$

where $\alpha$ is a constant and $I_0 = \exp(I'_N + \alpha N)$ represents the PL intensity of defect-free nanotubes.

Assuming stochastic formation of quenching sites with an average number $N$ in a single nanotube that recombine excitons nonradiatively, we have performed Monte Carlo simulation to quantify the effect of the quenching sites on the PL intensity from a CNT (see Refs. [4,5] for details). In the simulations, a nanotube length $L$ = 2 μm, a 1/e$^2$ laser beam radius $r$ = 400 nm (FWHM of ~470 nm), and an intrinsic exciton diffusion length $l$ = 700 nm are used, while excitons encountering nanotube edges, quenching sites, and other excitons recombine immediately.

Figure S7a shows simulated PL intensity as a function of $\lambda$, and the result is well fitted with Eq. S3 (red) for $\lambda > 3$ where the length of CNT segments is smaller than exciton diffusion length. Error bars represent the standard deviation, which originates from the random position of quenching sites as shown in Figure S7b. As discussed above, Monte Carlo simulation shows that the frequency of having $\lambda$ quenching sites follows a normal distribution (Figure S7c), and the histograms of PL intensity with different $N$ can be well fitted with a log-normal distribution (Figure S7d), in good agreement with the experiments. Note that the number of quenching sites $\lambda$ follows a Poisson distribution which can be approximated well by a normal distribution when the average number is large. Equation S1 does not hold for small $N$, resulting in the deviation from the fitting lines at large $I_{PL}$ as observed both in the experiments (the as-grown suspended CNTs and the CNTs on polystyrene) and the simulation ($N/L$ = 2 and 3 μm$^{-1}$). The $\log_{10}(I_{PL})$ of 5.6 (= 4×10$^5$ counts/s) in Figure S6 is therefore likely obtained from defect-free CNTs. We should also note that the following equation

$$I_{PL} = \sum_i^2 I_i \exp(-\alpha_i\lambda_i) \qquad \text{(S4)}$$

reproduces the result in Figure S7a better, and a histogram of $I_{PL}$ with this equation can be also fitted by a log-normal function over a wide range. Compared with the previously reported effective length dependence of PL quantum yield, where the quantum yield is

proportional to the square of effective tube lengths [6,7], Eqs. S3 and S4 fit the simulation result (Figure S7a) better and thereby the experimental $I_{PL}$ distribution (Figure S6a). This is probably because the tube segments separated by quenching sites have uneven lengths due to their random defect formation.

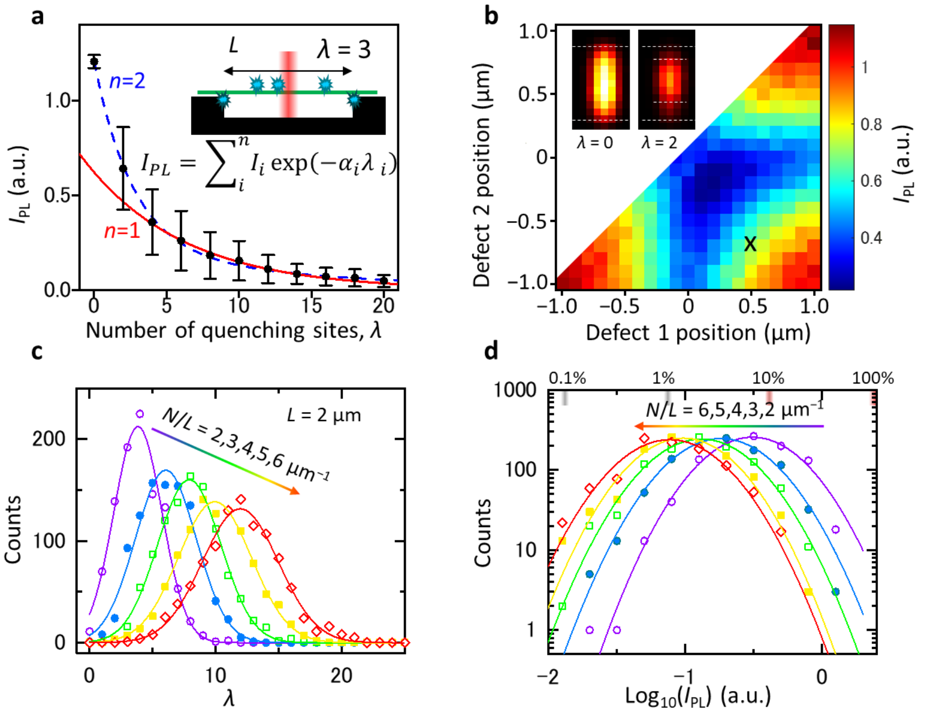


**Figure S7 | Monte Carlo simulation on PL intensity that depends on the number of quenching sites. a**, Simulated PL intensity as a function of the number of quenching sites $\lambda$ in a nanotube with a length $L$ of 2 µm. **b**, Simulated PL intensity as a function of the position of two quenching sites. Inset shows simulated confocal PL images without quenching sites and with two quenching sites at x in the color plot. **c**,**d** Histograms of $\lambda$ (**c**) and PL intensity (**d**) with different average densities of quenching sites ($N/L$). Excitation laser beam is fixed at the center of the nanotubes. The percentages at the top represent relative PL quantum yields compared to the intrinsic quantum yield of a sufficiently long CNT without quenching sites.

## S8. Influence of baking and water rinsing on PL properties

One of the major features of the anthracene-assisted transfer is the absence of high-temperature process and wet process. Anthracene crystals are removed typically at 110ºC, but this temperature can be lowered even to room temperature, though it takes a few days for the full sublimation. Also, the growth and the removal of anthracene crystals are conducted in gas phase, and no wet etching is required to peel the crystals off the substrate. When using polymer films to transfer CNTs [2], spin-coating of the polymer in solvents, etching of the growth substrates, and the removal of polymer by solvents or pyrolysis at high temperature are involved. We have compared the PL intensity of CNTs on PMMA

before and after baking at 170ºC, baking at 230ºC, and immersing in distilled water. In all cases, we find that the PL intensity decreased nearly by half (Figure S8). The linewidths also increased with these treatments. These results support the importance of avoiding high-temperature processes and wet processes in the anthracene-assisted transfer.

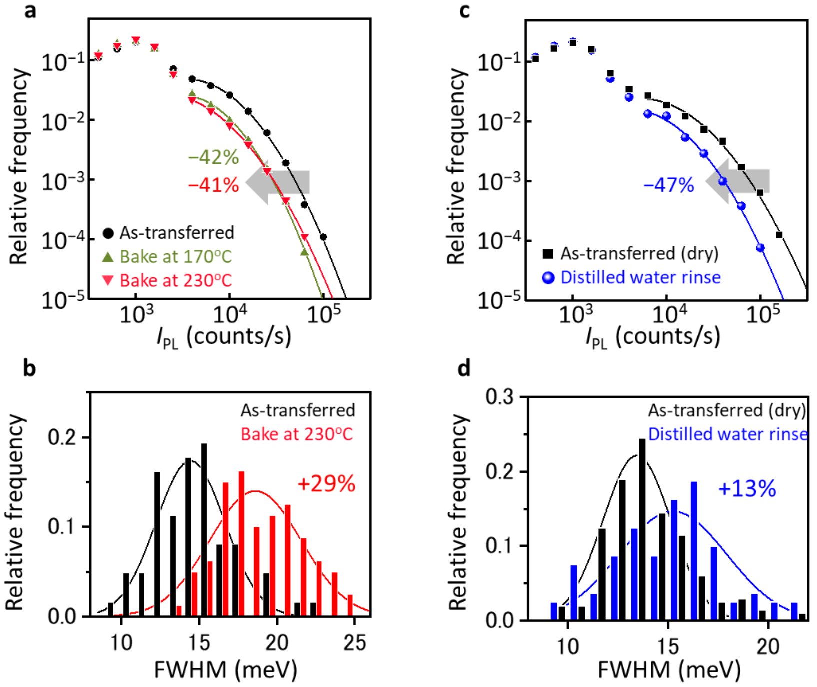


**Figure S8 | Effects of baking and water on PL. a**, $I_{PL}$ histograms of the CNTs transferred on PMMA. Black circles represent as-transferred CNTs, whereas green and red triangles represent the same sample but after bake at 170 and 230°C for 1 h, respectively. **b**, Spectral FWHM of as-transferred CNTs and those after the bake. **c**,**d**, Similar data set for as-transferred CNTs and the identical CNTs after the immersion in distilled water for 2 h. $P$ = 100 µW.

## S9. Anthracene-assisted transfer of monolayer $WSe_2$ over trenches

The advantages of using anthracene as sacrificial layers are also evident in the case of 2D materials, such as h-BN and $MoS_2$. We first prepared a flake of mechanically exfoliated $WSe_2$ onto a flat $SiO_2$/Si substrate (Figure S9a). A half of the $WSe_2$ flake is monolayer and another half is bilayer. This $WSe_2$ flake is then picked up on an anthracene crystal. Note that atomically flat surface of the anthracene crystal enhances the adhesion to 2D materials, and thereby enables the picking up of monolayer 2D materials from $SiO_2$/Si substrates.

We place the $WSe_2$/anthracene on a Si substrate with trenches, followed by sublimation of the anthracene crystal by mild heating, leaving behind the $WSe_2$ on the receiving substrate (Figure S9b). A dark-field image in Figure S9c shows that both monolayer and bilayer regions are suspended over the trenches. We have measured PL and Raman spectra from the monolayer (Figure S9d,f) and bilayer (Figure S9e,g) regions, and on the $SiO_2$/Si surface (green lines) and over the trench (red lines). When comparing the PL intensity of

the monolayer part, the suspended region shows significantly higher intensity than on the $SiO_2$/Si surface, while Raman spectra indicate negligible strain in the suspended region. The steep contrast of the PL intensity and spectral shape between Figure S9d and S9e originates from layer number difference. As the flatness and the sublimation of anthracene crystals facilitates the picking up of 2D materials and prevents surface tension from destroying the 2D materials, respectively, 2D materials transfer can be improved by this technique as much as 1D nanotubes.

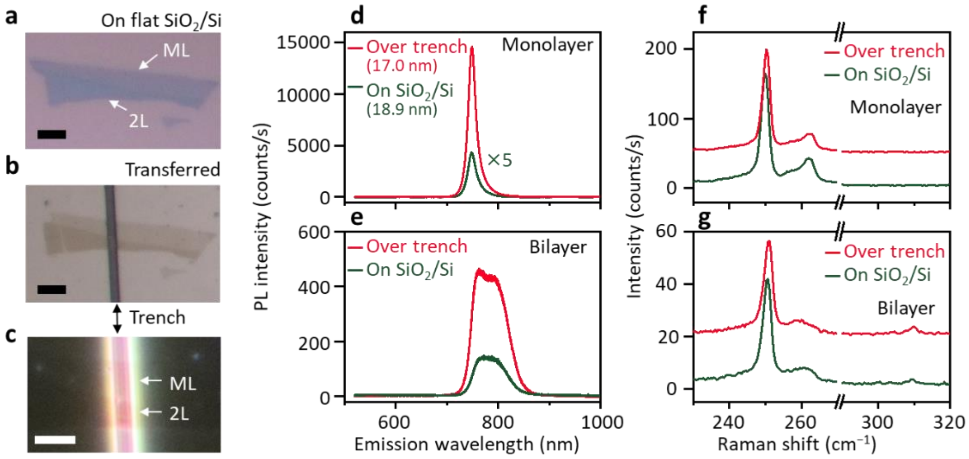


**Figure S9 | Anthracene-assisted transfer of monolayer WSe2. a**, Mechanically exfoliated mono- and bilayer $WSe_2$ on an $SiO_2$/Si substrate. **b**,**c**, Bright-field (**b**) and dark-field (**c**) optical images of the transferred $WSe_2$ flake on another $SiO_2$/Si substrate with a trench. All scale bars are 5 µm. **d**,**e**, PL spectra of the transferred $WSe_2$. Numbers in parentheses represent FWHM. The spectrum of the monolayer $WSe_2$ on an $SiO_2$/Si substrate is multiplied by 5 times for visual convenience. **f**,**g**, Raman spectra of the transferred $WSe_2$. Excitation wavelength for PL and Raman spectroscopy is 488 nm, and the excitation powers are 1.5 and 60 µW for PL and Raman spectroscopy, respectively.

## S10. Air-suspended CNTs prepared by polymer-mediated transfer

Polymer-mediated methods are often used to transfer CNTs onto flat substrates [2]. When there are trenches or slits in receiving substrates, the transferred CNTs tend to break or form bundles with neighboring CNTs due to the surface tension induced by organic solvents for polymer removal or molten polymers at high temperatures. In Figure S10c,d,e, the CNTs are transferred *via* a PMMA film, which has been formed by spin-coating of a 4wt% solution in anisole at 3000 rpm for 30 s. The PMMA film has been removed by annealing in Ar/$H_2$ atmosphere at 350°C for 6 h. Even when CNTs are still suspended after the polymer removal, the polymer remains on the CNTs, negatively influencing the PL properties (Figure S10f).

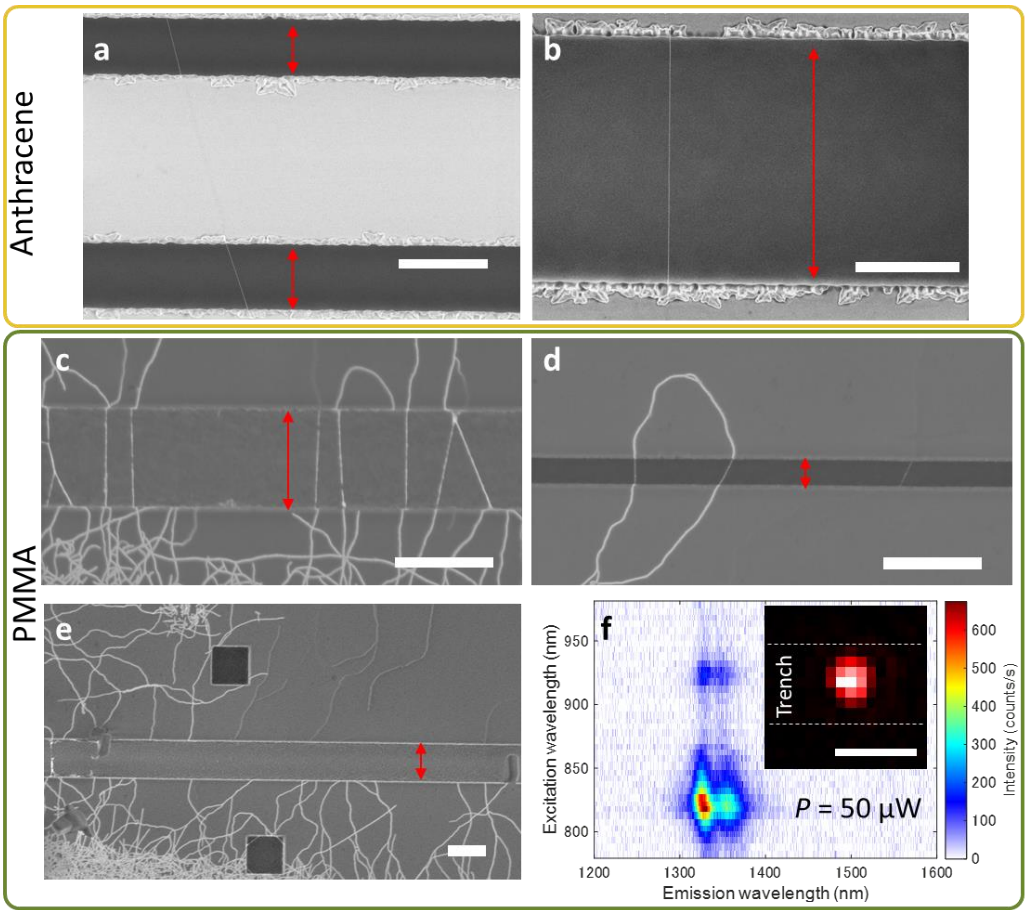


**Figure S10 | Comparison of CNTs transferred via anthracene and polymer. a–e**, Typical SEM images of air-suspended CNTs that are transferred *via* anthracene crystals (**a**,**b**) or *via* PMMA films (**c**–**e**). Red arrows represent the width of trenches. **f**, Typical PLE map for air-suspended CNTs by the PMMA transfer method. Inset: PL image of the CNT. All the scale bars are 2 μm.

## S11. Repeating deterministic transfer

After the (11,6) nanotube was transferred (Figure 4b,c), we transferred a (9,7) CNT nearby. In Figure S11b, PL signals at the emission wavelengths $\lambda_{ex}$ of 1330 and 1433 nm are shown in green and red, respectively, and the laser reflectivity is superimposed in gray scale. Polarization dependence of $I_{PL}$ in the inset of Figure S11b indicates the angle between these tube axes to be ~60 degrees. Figure S11c,d display the PL emission spectra excited at each $E_{22}$ resonance and PLE spectra cut at each $E_{11}$ peak, respectively. These spectra are measured at the same spot, confirming the presence of both (9,7) and (11,6) tubes at the designated position. The (9,7) tube is located even closer to the center of the cross mark than the other tube, indicating the position accuracy in our transfer system.

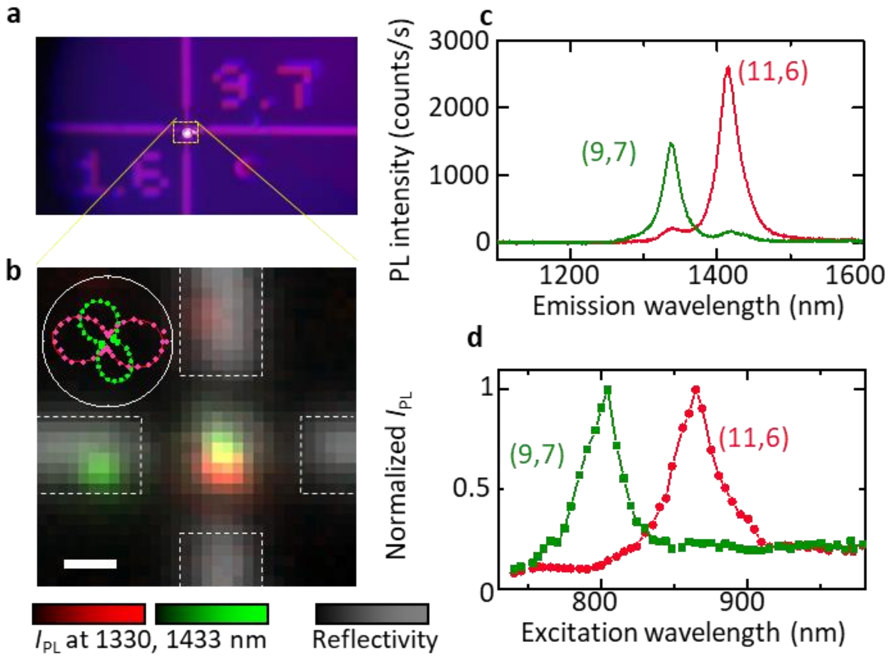


**Figure S11 | Multiple transfer of chirality-selected CNTs to a designated position. a**, Wide-field optical image of a target substrate during the second transfer process. Numbers, such as (9,7) and (11,6), are lithographically patterned metals, and represent the chiral indices of CNTs to be transferred. Bright spot near the center is the laser beam reflection, where PL spectra is obtained in real time for the alignment. **b**, Confocal PL image of transferred CNTs. Intensities at 1330 and 1433 nm, and laser reflectivity are colored in red, green, and gray, respectively. Scale bar is 1 µm. Inset: Polarization dependence of $I_{PL}$. **c**,**d**, PL emission spectra (**c**) and PL excitation spectra (d) of the transferred CNTs. $P$ = 100 µW and laser polarization is parallel to each CNT.

## S12. PL properties after the first and the second transfer processes

In Figure 5, the (10,5) and (13,5) CNTs are transferred in sequence. The characteristics of the (10,5) tube along are shown here in comparison with those after the transfer of the (13,5) tube. When comparing the PL images in Figure 5b and Figure S12a, there is no obvious difference before and after the transfer of the (13,5) tube. Before the second transfer process, there is no emission at ~1500 nm, as evidenced by Figure S12b,c.

To estimate the exciton transfer efficiency from the (10,5) tube to the (13,5) tube, we first extract the contribution of intertube exciton transfer to the total PL intensity by subtracting Figure 5a from Figure 5c with a coefficient of 0.294 (Figure S12d). Here, the PL intensity from the region far from the junction (exciton generation through the off-resonant photon absorption) is cancelled out. Taking the ratio of the PL intensities in Figures S12d to 5c, the contribution of the intertube exciton transfer to the (13,5) tube emission is 42% from this simple estimation. Then, we calculate the fraction of the (13,5)

tube emission due to the excitons generated in the (10,5) tube and transferred to the (13,5) tube with respect to the total intensity. Using $I_{PL}$ centered at 1263 nm ($1.27\times10^5$ counts/s) and 1514 nm ($0.26\times10^5$ counts/s) at the blue diamond in Figure 5b,c, the transfer efficiency is calculate to be 7.8% ($=0.42\times0.26\times10^5/(0.42\times0.26\times10^5+1.27\times10^5)$). Note that exciton-exciton annihilation and the difference in the PL quantum yield of each CNT affect the estimation of the exciton transfer efficiency, but these factors are ignored for simplicity.

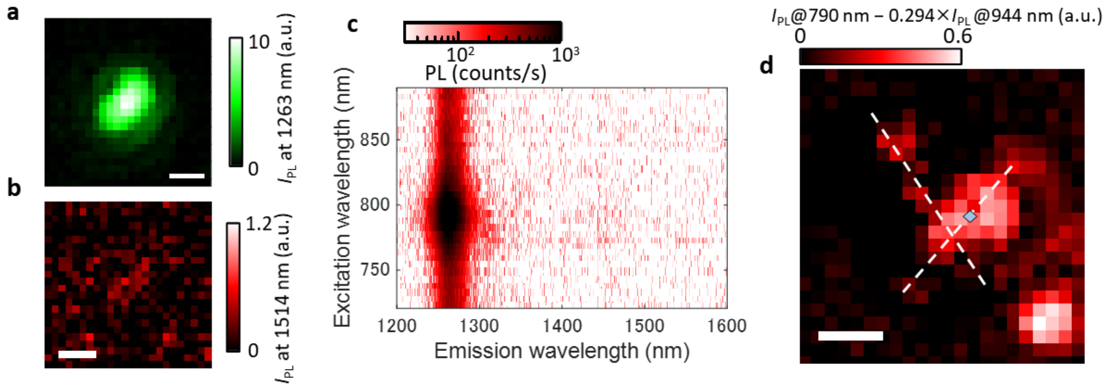


**Figure S12 | PL before and after the junction formation. a,b,** PL image of the (10,5) CNT in Figure 5 in the main text before the cross junction formation with the spectral windows centered at 1263 nm (**a**) and 1514 nm (**b**). **c,** PLE map for the CNT shown in **a**. **d,** Extracted PL image of the (13,5) tube obtained from Figures 5a,c, which shows the contribution of the intertube exciton transfer to the PL emission. Scale bars are 1 μm.

## S13. Periodic strain induced during the CNT growth

In Figure 5d,e, PL emission from the (13,5) tube is split into two peaks because of strong local strain that has been created during the CNT growth on quartz [8] (see Figure S13a,b). The strain is induced by the difference in thermal expansion coefficients between CNTs and the quartz substrates, and results in the energy shift at $E_{ii}$ resonances and Raman spectra, *e.g.* G-band shifts as shown in Figure S13c. For example, the PL emission peaks can be different by ~100 nm within a single nanotube. Surprisingly, such strain is preserved all the way through the transfer process if the entire length of CNTs remains in contact with the supporting substrates, which is not observed for the polymer-mediated wet transfer technique [2,9]. Difference in G-peak frequency within the transferred nanotube is as large as 12 $cm^{-1}$ (Figure S13d), corresponding to $E_{11}$ energy shift of ~45 meV when the same relation between G-peak position and $E_{11}$ energy (3.72 meV/$cm^{-1}$) is assumed.

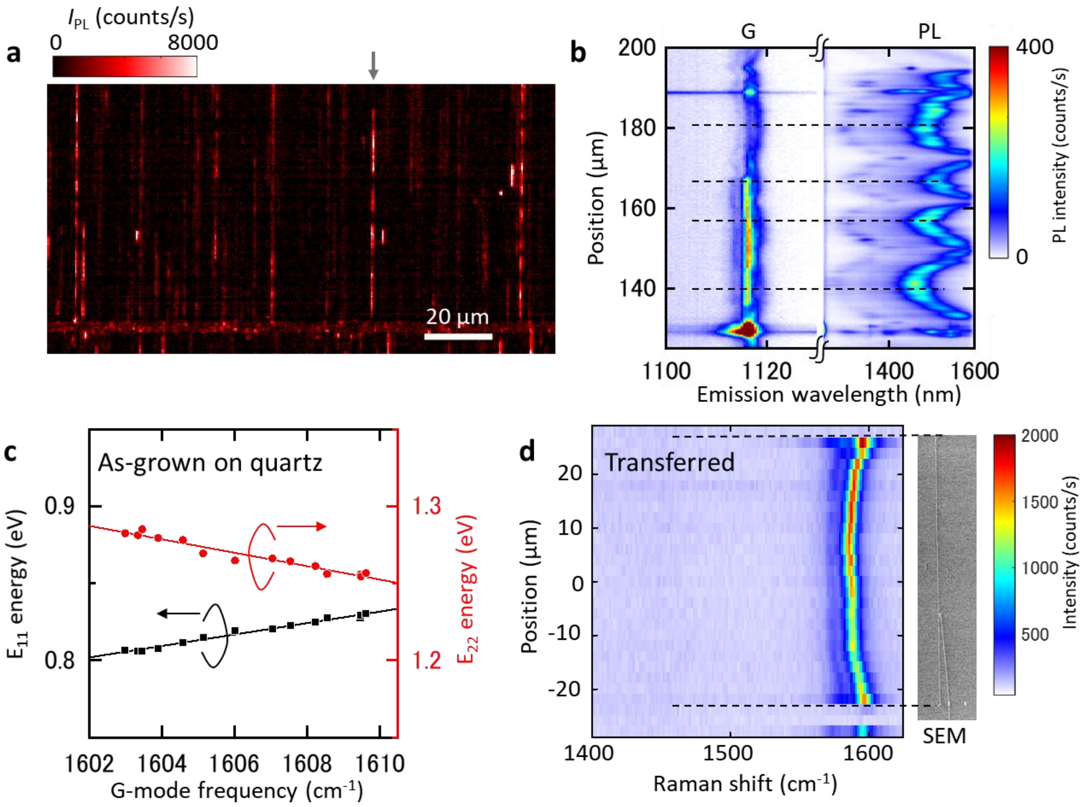


**Figure S13 | Strain induced during the CNT growth.** **a**, PL image of as-grown CNTs on quartz substrate. $I_{PL}$ is integrated at 1498 nm with a spectral window of 50 nm. $P$ = 1.2 mW. **b**, PL (and Raman) intensity map along the single CNT indicated by the arrow in **a**. Not that there could be multiple CNTs within an excitation laser spot when G-band appears. **c**, $E_{11}$ and $E_{22}$ energies as a function of the peak position of G-band for the CNT shown in **a** and **b**. **d**, Raman intensity map along a transferred CNT from quartz.

## REFERENCES


S1. Ye, X. *et al.* Microspacing In-Air Sublimation Growth of Organic Crystals. *Chem. Mater.* **30**, 412–420 (2018).

S2. Jiao, L. *et al.* Creation of nanostructures with poly(methyl methacrylate)-mediated nanotransfer printing. *J. Am. Chem. Soc.* **130**, 12612–12613 (2008).

S3. Schweiger, M., Zakharko, Y., Gannott, F., Grimm, S. B. & Zaumseil, J. Photoluminescence enhancement of aligned arrays of single-walled carbon nanotubes by polymer transfer. *Nanoscale* **7**, 16715–16720 (2015).

S4. Ishii, A., Yoshida, M. & Kato, Y. K. Exciton diffusion, end quenching, and exciton-exciton annihilation in individual air-suspended carbon nanotubes. *Phys. Rev. B* **91**, 125427 (2015).

S5. Otsuka, K., Ishii, A. & Kato, Y. K. Super-resolution fluorescence imaging of carbon nanotubes using a nonlinear excitonic process. *Opt. Express* **27**, 17463 (2019).
S6. Hertel, T., Himmelein, S., Ackermann, T., Stich, D. & Ḱ, J. C. Diffusion Limited Photoluminescence Quantum Yields in 1-D Semiconductors : *ACS Nano* **4**, 7161–7168 (2010).
S7. Harrah, D. M. & Swan, A. K. The Role of Length and Defects on Optical Quantum Efficiency and Exciton Decay Dynamics in Single-Walled Carbon Nanotubes. *ACS Nano* **5**, 647–655 (2011).
S8. Ozel, T., Abdula, D., Hwang, E. & Shim, M. Nonuniform Compressive Strain in Horizontally Aligned Single-Walled Carbon Nanotubes Grown on Single Crystal Quartz. *ACS Nano* **3**, 2217–2224 (2009).
S9. Otsuka, K. *et al.* Digital Isotope Coding to Trace the Growth Process of Individual Single-Walled Carbon Nanotubes. *ACS Nano* **12**, 3994–4001 (2018).
